# Supplementary material for: Towards Real-World Blind Face Restoration with Generative Facial Prior
Source: arXiv:2101.04061 source file (2021-06-11)
Supplement: Supplementary file 1 [file 5_appendix.tex]

% !TEX root = ../main.tex

\noindent\textbf{\large{Appendix}} \label{appendix}

\vspace{0.1cm}
\textit{
	We first provide more details about filter analyses on other tasks in 
	Sec.~\ref{sec:filter_analyses}, such as super-resolution with different kernels and JPEG artifacts removal with 
	different compression qualities.
	% The phenomenon of non-linearity between interpolation coefficients and effects is illustrated in 
	% Sec.~\ref{subsec:non-linearity}.
	We then provide the implementation details of deep network interpolation for different applications in  
	Sec.~\ref{sec:implementation_details}.
	Additional applications and analyses are presented in Sec.~\ref{sec:more_applications_and_analyses}. 
}

%%%%%%%%% BODY TEXT
\section{Filter Analyses} \label{sec:filter_analyses}
%\subsection{Similar Observations on Several Tasks}
In the main paper, we provide a preliminary explanation behind the deep network interpolation (DNI) from the filter 
perspective, through analyses of the denoising task. Specifically, the observations can be summarized as:
1) Fine-tuning facilitates high correlation between parameters of different networks, providing the possibility for 
meaningful interpolation. 2) Fine-tuned filters for a series of related tasks present continuous changes. 3) Our 
analyses show that interpolated filters could fit the actual learned filters well.

The similar observations could also be found in several other tasks, such as super-resolution with different kernels 
and JPEG artifacts removal with different compression levels. In particular, we also adopt a three-layer network 
similar to SRCNN~\cite{dong2014learning}, where the first and last convolutional layers have 9$\times$9 filter size 
(\ie, the 
same architecture as that in the main paper). Following the notion of~\cite{dong2014learning}, the first and last 
layer can be viewed as a \textit{feature extraction} and \textit{reconstruction} layer, respectively.

For super-resolution, we focus on a series of blurring kernels with 
different kernel widths, followed by a down-sampling operation. The kernel widths in our experiments are K3, K5, K7, 
K9, and K11, where K3 denotes a Gaussian blur kernel with size 3. We use the \textit{OpenCV GaussianBlur} 
function and the Gaussian kernel standard deviation can be derived from the kernel width.

For JPEG compression artifacts removal, we employ increasing compression qualities with Q10, Q20, Q30, Q40, and Q50, 
(the larger the number, the better image quality after compression).

We obtain all the models from one pre-trained model by fine-tuning. The fine-tuning maps are depicted in 
Fig.~\ref{fig:model_finetune}. Each dot in the figure represents a model. Lines with arrows denote fine-tuning. For 
instance, the super-resolution (K3) model is fine-tuned from the denoising (N20) model. 

\begin{figure}[h]
	\begin{center}
		%\fbox{\rule{0pt}{4.45in} \rule{1\linewidth}{0pt}}
		\includegraphics[width=\linewidth]{figs/model_finetune.pdf}
		\caption{Each dot represents a model.  Lines with arrows denote fine-tuning. For instance, the 
		super-resolution (K3) model is fine-tuned from the denoising (N20) model. 
		}
		\label{fig:model_finetune}
	\end{center}
	\vspace{-0.7cm}
\end{figure}

\begin{figure*}[th]
	\begin{center}
		%\fbox{\rule{0pt}{4.45in} \rule{1\linewidth}{0pt}}
		\includegraphics[width=\linewidth]{figs/filter_denoise_sr_dejpeg.pdf}
		\caption{Filter visualization examples of the \textit{feature extraction} and \textit{reconstruction} layers 
			for denoising, super-resolution and DeJPEG tasks. 1) The learned filters for different 
			distortion levels under the same degradation exhibit continuous changes. 2) Filters 
			for different image distortions (\eg, denoising and super-resolution) capture the special 
			characteristics of their own tasks, representing different filter patterns, especially in the 
			\textit{reconstruction} layer.
		}
		\label{fig:filter_denoise_sr_dejpeg}
	\end{center}
	\vspace{-0.3cm}
\end{figure*}

\begin{figure*}[th]
	\begin{center}
		%\fbox{\rule{0pt}{4.45in} \rule{1\linewidth}{0pt}}
		\includegraphics[width=\linewidth]{figs/filter_cor.pdf}
		\caption{Filter correlation index curves of the \textit{feature extraction} and \textit{reconstruction} layers 
			for denoising, super-resolution and DeJPEG tasks. The curves present the median of correlation 
			indexes and the correlation distributions are also plotted. These curves show that the learned filters for 
			different distortion levels under the same distortion exhibit continuous changes. 
		}
		\label{fig:filter_cor}
	\end{center}
	\vspace{-0.3cm}
\end{figure*}
 
Fig.~\ref{fig:filter_denoise_sr_dejpeg} visualizes several filter examples of the feature extraction and 
reconstruction layers for denoising, super-resolution and DeJPEG tasks.
We can found that: 1) Under the constraint of fine-tuning, the learned 
filters for related tasks exhibit continuous changes. This phenomenon is observed in all the tasks, including 
denoising, super-resolution and DeJPEG.
2) Except the similarity, we further see that filters for different image 
distortions (\eg, denoising and 
super-resolution) capture the special characteristics of their own tasks, representing different filter patterns, 
especially in the reconstruction layer.
Thus, if two tasks are far way from each other, the weak correlation of filters 
could result in unsatisfying, even meaningless interpolated results.
The definition of task distances and the application boundaries of DNI are still open questions. Our analyses focus on 
related tasks of different degradations under the same distortion. It is noteworthy that DNI is capable of dealing with 
lot of tasks for continuous imagery effect transition and its broad applications indicate that related tasks with close 
``distances'' are common and practical in real-world scenarios.

\begin{figure*}[th]
	\centering
	\vspace*{2mm}\begin{subfigure}[b]{0.95\linewidth}
		\includegraphics[width=\linewidth]{figs/interp_filter_cor1.pdf}
		\vspace*{-7mm}\caption{The \textit{feature extraction} layer (first layer).}
	\end{subfigure}
	\\
	\vspace*{2mm}\begin{subfigure}[b]{0.95\linewidth}
		\includegraphics[width=\linewidth]{figs/interp_filter_cor1.pdf}
		\vspace*{-7mm}\caption{The \textit{reconstruction} layer (last layer).}
	\end{subfigure}
	\vspace*{-2mm}
	\caption{The correlation curves for actual learned filters and interpolated filters are very 
		close for both the \textit{feature extraction} and \textit{reconstruction} layers, indicating that the 
		interpolated filters could fit learned filters well.
		The similar observations could be found on denoising, super-resolution and DeJPEG tasks.
	}
	\label{fig:interp_filter_cor}
	\vspace*{0mm}
\end{figure*}

We also calculate the filter correlation indexes and plot their correlation distribution. The curves of the 
\textit{feature extraction} and \textit{reconstruction} layers for denoising, super-resolution and DeJPEG tasks are 
shown in Fig.~\ref{fig:filter_cor}. We again observe continuous changes of learned filters for different distortion 
levels under the same distortion.

We then show that the interpolated filters fit the learned filters well for different layers in the networks, and 
also for different tasks including denoising, super-resolution and DeJPEG.
We perform linear interpolation between the filters from the two ends of degradation levels (\eg, the N20 and N60
models for denoising; the K3 and K11 models for super-resolution).
With optimal interpolation coefficients $\alpha$, the interpolated filters could visually fit those learned filters for 
all the three 
tasks, as shown in Fig.~\ref{fig:interp_filter_cor}. The observations could 
be held for both the feature extraction and reconstruction layers. 

The optimal $\alpha$ is obtained through the final performance of the interpolated 
network. Specifically, we perform DNI with $\alpha$ from 0 to 1 with an interval of 0.05. The best $\alpha$ for
each degradation level is selected based on the highest PSNR on the
test dataset.

As the network goes deeper, the non-linearity increases and the network behaviors become more complicated. We provide a 
preliminary analysis of deeper denoising network in the main paper, where the observations are consistent with our 
conclusion.
For other tasks, such as image style transfer or image translation, the investigation from the filter perspective 
becomes more sophisticated, since these tasks cannot be defined continuously like the continuous degradation levels
in image restoration. 
The exploration of inherent filter correlations and the in-depth reason why DNI works are worth investigated in the
future work.

\vspace{3mm}
%\subsection{The Non-linearity between Interpolation Coefficients and Effects}\label{subsec:non-linearity}
\noindent\textbf{The non-linearity between interpolation coefficients and effects.}
%% the nonliearn relation between the coefficients and the effects 
In our analyses, in order to realize ``linear effects'' of outputs, (\ie obtaining denoising models dealing with 
N30, N40 and N50), the different interpolation coefficients do not present a linear relationship. The practical 
optimal $\alpha$, obtained through the final performance of the interpolated 
network, for each noise level is shown in Fig.~\ref{fig:interp_nonlinear} (orange curve).
One reason is that the effects of filter interpolation and the output effects are inherently not linear.
We can also obtain the optimal $\alpha$ by optimizing the filter correlation index with models trained for each 
noise levels.
A similar non-linear trend as the practical curve could be observed (Fig.~\ref{fig:interp_nonlinear}, green curve).
We suspect that the extra gap between the green and orange curves may be from the non-linearity in networks.

The non-linear sampling of $\alpha$ for ``linear'' transition effects could be observed in many DNI applications. 
However, it does not 
influence its extensive applications. A solution is to control the sampling density of $\alpha$, simply resulting in 
``linear'' transition effects. 

\begin{figure}[h]
	\begin{center}
		%\fbox{\rule{0pt}{4.45in} \rule{1\linewidth}{0pt}}
		\includegraphics[width=\linewidth]{figs/interp_nonlinear.pdf}
		\caption{To achieve ``linear'' transition effects, the coefficients for each level are non-linear both from 
			ideal analyses (optimizing the filter correlation) and practical performance (obtaining from the final 
			PSNR.) 
		}
		\label{fig:interp_nonlinear}
	\end{center}
\end{figure}

\section{Implementation Details}\label{sec:implementation_details}
In this section, we provide the implementation details of DNI and the fine-tuning strategy for several applications in the main 
paper.

\noindent\textbf{Balance MSE and GAN effects in super-resolution.}
The MATLAB bicubic kernel with a scaling factor of 4 is adopted as the down-sampling kernel.
We first train a super-resolution model with MSE loss~\cite{timofte2017ntire}, which tends to produce over-smooth 
images.
We then fine-tune it with GAN loss and perceptual loss~\cite{ledig2017photo}, obtaining results with vivid details yet 
accompanied with unpleasant artifacts.
DNI is applied in these two models. 
We use dense blocks~\cite{huang2016densely} as the network architecture.

\noindent\textbf{Image-to-image Translation.}
In image-to-image translation, we use the popular CycleGAN~\cite{zhu2017unpaired} to explore the broad applications of 
DNI\footnote{We use the official released 
codes: \url{https://github.com/junyanz/pytorch-CycleGAN-and-pix2pix}.}.
In the original CycleGAN, there are two networks $G_A$ and $G_B$ to learn a mapping and its inverse mapping, 
respectively. For 
instance, in order to translate landscape photos to paintings, $G_A$ learns the mapping from paintings 
to photos while $G_B$ learns an inverse mapping from photos to painting.

We use slightly different settings for different applications. For \textit{mixing various painting styles}, we first 
train a 
CycleGAN model for translating photos to paintings with Van Gogh's style, \ie, $G_A^{Van Gogh}$ is used for turning Van 
Gogh paintings into photos, and $G_B^{Van Gogh}$ for translating photos into paintings with Van Gogh's style. 
We then fine-tune these two networks $G_A^{Van Gogh}$ and $G_B^{Van Gogh}$ (together with the discriminators) to models 
with another painter style, such as Monet, and obtain $G_A^{Monet}$ and $G_B^{Monet}$. 

During inference, our aim is to translate a landscape photo to paintings with various styles, even the mixtures of 
several famous painters. Thus, we only keep the $G_B^{Van Gogh}$ and $G_B^{Monet}$ and perform DNI on these 
two networks.

For \textit{day-to-night application}, we first train a CycleGAN model as usual, \ie, $G_A$ is used for translating a 
day photo to a night one while $G_B$ translates the night photo to the day one. Note that the CycleGAN model is only 
able to translate between two states and cannot produce a series of images with smooth transitions from day to night.
We then fine-tune the whole pre-trained model with identity mapping. Specifically, we remove the GAN loss, adopt a 
$10\times$ identity loss and keep the cyclic loss in the CycleGAN framework. Thus, the fine-tuned network 
$G_A^{identity}$ 
always outputs identical results, \ie, it receives a day photo and outputs the same day photo.

DNI is then applied in $G_A$ and $G_A^{identity}$. With an appropriate coefficient, the interpolated network is able to 
produce images with arbitrary effects between day and night. The same operations are also employed in the 
\textit{deep-to-shallow depth of filed} application.

\noindent\textbf{Style Transfer.}
We use the PyTorch example codes for style 
transfer\footnote{\url{https://github.com/pytorch/examples/tree/master/fast_neural_style}.}.
We first train a model for one certain style and then fine-tune it for another style. DNI is performed on these two 
models. For the stroke factor, we fine-tune the pre-trained model for a style image with different size.
In order to balance the content and style, we fine-tune 
the pre-trained model with smaller style loss, resulting in almost identity mapping.

We note that DNI is generic for several controllable factors in style transfer, such as styles, strokes, and the balance of 
content and style. The proposed DNI could be also applied to more advanced models~\cite{dumoulin2016learned,huang2017arbitrary}
that address multiple or arbitrary style transfer, resulting in more diverse outputs.

\section{More Applications and Analyses}\label{sec:more_applications_and_analyses}

\subsection{Extend Restoration Models to Unseen Distortion Levels}

\begin{figure*}[th]
	\begin{center}
		%\fbox{\rule{0pt}{4.45in} \rule{1\linewidth}{0pt}}
		\includegraphics[width=\linewidth]{figs/denoise_interp.pdf}
		\caption{Extending denoising models to unseen noise levels. The baseline model trained with N20 and N60 data is 
			incapable of removing unseen noise (\eg, N30 and N40), while our method  could deal with these 
			unseen scenes. 
			(\textbf{Zoom in for best view})}
		\label{fig:denoise_interp}
	\end{center}
	\vspace*{-5mm}
\end{figure*}

In Sec.~\ref{sec:filter_analyses}, we reveal the inherent correlation of learned filters for a series of related 
tasks. Here, we take advantage of this observation to extend restoration models to deal with unseen distortion 
levels. We take the denoising task for example and it could also be applied to other restoration tasks, \eg, 
super-resolution with different down-sampling kernels. 

%% settings 
We employ an extreme case, where only the data with noise level N20 and N60 are available during training 
and we expect the trained models are able to handle arbitrary noise levels in the middle during testing. In particular, 
we test unseen N30, N40, and N50 noise levels.
The upper bound for each level is the model trained with its corresponding data. The baseline is the model trained with 
both the N20 and N60 data.
% structure
We adopt DnCNN~\cite{zhang2017beyond} as the denoising model\footnote{We use the official released 
codes:\url{https://github.com/cszn/DnCNN} (PyTorch version).} and use two variants, with and without BN. 
% Different from the shallow 
% models for analyses in Sec.~\ref{subsec:filter_analysis}, DnCNN is a deeper model with 17 convolutional layers.

% our method
We first train a model using N20 data and then fine-tune it with N60 data. DNI is then performed with interpolation 
coefficients $\alpha \in [0, 1]$ with an interval of 0.1. 
The best result for each noise level is selected among these interpolated models (the chosen $\alpha$ for each level 
is shown in Tab.~\ref{tb:DnCNN_denoise}). 
We note that the selection is simple with a few trials due to the smooth transition. For automatic denoising, we could 
further train a shallow network to regress a proper $\alpha$ according to the noisy input.

% evaluate
We evaluate DNI using the LIVE1~\cite{sheikh2005live} dataset. Quantitative results with the PSNR metric
and qualitative results are shown in Tab.~\ref{tb:DnCNN_denoise} and Fig.~\ref{fig:denoise_interp} respectively.
The baseline model is incapable of removing unseen noise (\eg, N30 and N40 in Fig.~\ref{fig:denoise_interp}), leading 
to drastic drops in performance. However, our method could deal with those unseen scenes, even approaching 
to the upper bound. (Note that the upper bound observes the corresponding data.)

Though our DNI with BN can outperform its corresponding baseline, there is still a little drop compared with that 
without BN. The BN effects for DNI are still an open question and a better interpolation scheme needs to be explored 
for normalization layers. 
We also note that this application demonstrates that it is worth exploiting the underlying relations of learned 
filters to further extend the ability and practicality of existing models.

\begin{figure*}[th]
	\begin{center}
		%\fbox{\rule{0pt}{4.45in} \rule{1\linewidth}{0pt}}
		\includegraphics[width=\linewidth]{figs/denoise_spatial_control.pdf}
		\caption{Spatial control for adjustable denoising.
			With a mask, different denoising strengths are applied separately for the foreground and the background. 
			(\textbf{Zoom in for best view})}
		\label{fig:denoise_spatial_control}
	\end{center}
	\vspace*{-5mm}
\end{figure*}

\begin{table}[htbp]
	\centering
	\caption{The average denoising results of PSNR (dB) on the LIVE1 test dataset. Unseen noise levels are denoted with 
		*. Note that the upper bound have seen the corresponding data.}
	\label{tb:DnCNN_denoise}
	\tabcolsep=0.16cm
	\begin{tabular}{cc|ccccc}
		\hline
		& Noise level  & N20  & N30*  & N40*  & N50*  & N60  \\ \hline \hline
		
		\multicolumn{1}{c|}{\multirow{4}{*}{\rotatebox{90}{w/o BN}}}
		& Upper bound  & 32.38  & 30.39  & 29.01  & 27.98  & 27.18  \\
		\multicolumn{1}{c|}{}
		& Baseline  & 32.36  & 23.86  & 21.90  & 27.34  & 27.14  \\
		\multicolumn{1}{c|}{}
		& \textbf{DNI (ours)} & \textbf{32.38} & \textbf{29.84} & \textbf{28.28} & \textbf{27.67} & \textbf{27.18} \\
		\multicolumn{1}{c|}{}
		& $\alpha$  & 1  & 0.7  &  0.4  & 0.1  & 0  \\ \hline \hline
		
		\multicolumn{1}{c|}{\multirow{4}{*}{\rotatebox{90}{w/ BN}}}
		& Upper bound  & 32.49  & 30.48  & 29.09  & 27.96  & 27.25  \\
		\multicolumn{1}{c|}{}
		& Baseline  & 32.42  & 24.42  & 26.58  & 27.44  & 27.21  \\
		\multicolumn{1}{c|}{}
		& \textbf{DNI (ours)} & \textbf{32.49} & \textbf{29.46} & \textbf{28.08} & \textbf{27.66} & \textbf{27.25} \\
		\multicolumn{1}{c|}{}
		& $\alpha$  & 1  & 0.6  & 0.3  & 0.1  & 0  \\ \hline
	\end{tabular}
	\vspace*{-5mm}
\end{table}

\if 0
\noindent\textbf{Super-resolution with different kernel sizes}
\begin{table}[htbp]
	\centering
	\caption{The average super-resolution ($\times 4$) results of PSNR (dB) on the Set14 test dataset. Unseen kernel 
		widths are denoted with *. (a modified SRResNet architecture).}
	\label{tb:SRResNet_sr}
	\begin{tabular}{c|ccccc}
		\hline 
		Kernel width  & K3  & K5*  & K7*  & K9*  & K11  \\ \hline \hline
		Upper bound   & 26.20  & 26.51  & 26.74  & 26.82  & 26.86  \\
		Baseline      & 26.17  & 26.24  & 25.49  & 25.39  & 26.78  \\
		DNI (ours)    & \textbf{26.20} & \textbf{26.47} & \textbf{26.66} & \textbf{26.76} & \textbf{26.86} \\
		$\alpha$      & 1  & 0.8  & 0.5  & 0.3  & 0  \\ \hline
	\end{tabular}
\end{table}
\fi

\subsection{Spatial Control for Adjustable Denoising}
In the main paper, we emphasize the importance of adjustable denoising strength and show the ability of DNI to satisfy 
the needs.
Here, we further present an application of spatial control for adjustable denoising. For the DSLR photos with shallow 
depth-of-filed, the background is usually blurred while the foreground contains rich details. We can easily separate 
them with a mask and adopt different denoising strengths respectively, obtaining better visual quality.
From Fig.~\ref{fig:denoise_spatial_control}, we can see that with adjustable denoising realized by DNI, the blurry area 
is more smooth without artifacts, while there are rich details in texture regions.

Apart from the denoising task, the adjustments with DNI can also be applied to other image restoration tasks, \eg, 
super-resolution with different down-sampling kernels and JPEG artifacts removal with different compression qualities.

\subsection{Multi-ends DNI}
A general form of DNI is also capable of interpolating more than two networks. 
Fig.~\ref{fig:painting_multi_ends} shows two examples of translating landscape photos to paintings with various 
styles -- Van Gogh, C\'ezanne, Monet and Ukiyo-e. By adjusting the interpolated coefficients, richer and more diverse 
effects with continuous transitions could be realized.

Another example of image style transfer in Fig.~\ref{fig:styles} presents the ability of DNI to transfer among 
different styles -- Mosaic style, Candy style, Mondrian style and Udnie style. It generates diverse and new styles, 
meeting users' various aesthetic flavors. 

\begin{figure*}[th]
	\centering
	\vspace*{2mm}\begin{subfigure}[b]{\linewidth}
		\includegraphics[width=\linewidth]{figs/painting_multi_ends_2.pdf}
		%\vspace*{-4mm}\caption{Denoising (N20)}
	\end{subfigure}
	\\
	\vspace*{2mm}\begin{subfigure}[b]{\linewidth}
		\includegraphics[width=\linewidth]{figs/painting_multi_ends_1.pdf}
		%\vspace*{-4mm}\caption{Super-resolution (K3)}
	\end{subfigure}
	\vspace*{-5mm}
	\caption{(Two examples) Translating landscape photos to paintings with various 
		styles -- Van Gogh, C\'ezanne, Monet and Ukiyo-e. By adjusting the interpolated coefficients, richer and more
		diverse effects with continuous transitions could be realized.
	}
	\label{fig:painting_multi_ends}
	\vspace*{0mm}
\end{figure*}

\begin{figure*}[h]
	\begin{center}
		%\fbox{\rule{0pt}{4.45in} \rule{1\linewidth}{0pt}}
		\includegraphics[width=0.98\linewidth]{figs/style.pdf}
		\caption{Image style transfer among different styles -- Mosaic style, Candy style, Mondrian style and Udnie 
		style. It generates diverse and new styles, meeting users' various aesthetic flavors. 
		}
		\label{fig:styles}
	\end{center}
	\vspace*{-4mm}
\end{figure*}

\if 0

\begin{figure*}[b]
	\centering
	\vspace*{2mm}\begin{subfigure}[b]{\linewidth}
		\includegraphics[width=\linewidth]{figs/filter_denoise_N20_conv0.png}
		\vspace*{-4mm}\caption{Denoising (N20)}
	\end{subfigure}
	\\
	\vspace*{2mm}\begin{subfigure}[b]{\linewidth}
		\includegraphics[width=\linewidth]{figs/filter_SR_K3_conv0.png}
		\vspace*{-4mm}\caption{Super-resolution (K3)}
	\end{subfigure}
	\\
	\vspace*{2mm}\begin{subfigure}[b]{\linewidth}
		\includegraphics[width=\linewidth]{figs/filter_deJPEG_Q50_conv0.png}
		\vspace*{-4mm}\caption{DeJPEG (Q50)}
	\end{subfigure}
	\vspace*{-5mm}
	\caption{Filter visualization of the \textit{feature extraction layer} (the first layer) for denoising (N20), 
	super-resolution (K3), and deJPEG (Q50) tasks. The K3 and Q50 models are fine-tuned from the N20 model.
	}
	\label{fig:filter_all_conv0}
	\vspace*{0mm}
\end{figure*}

\begin{figure*}[th]
	\centering
	\vspace*{2mm}\begin{subfigure}[b]{\linewidth}
		\includegraphics[width=\linewidth]{figs/filter_denoise_N20_conv2.png}
		\vspace*{-4mm}\caption{Denoising (N20)}
	\end{subfigure}
	\\
	\vspace*{2mm}\begin{subfigure}[b]{\linewidth}
		\includegraphics[width=\linewidth]{figs/filter_SR_K3_conv2.png}
		\vspace*{-4mm}\caption{Super-resolution (K3)}
	\end{subfigure}
	\\
	\vspace*{2mm}\begin{subfigure}[b]{\linewidth}
		\includegraphics[width=\linewidth]{figs/filter_deJPEG_Q50_conv2.png}
		\vspace*{-4mm}\caption{DeJPEG (Q50)}
	\end{subfigure}
	\vspace*{-5mm}
	\caption{Filter visualization of the \textit{reconstruction layer} (the last layer) for denoising (N20), 
		super-resolution (K3), and DeJPEG (Q50) tasks. The K3 and Q50 models are fine-tuned from the N20 model.
		Compared with the \textit{feature extraction layer} (the first layer) (Fig.~\ref{fig:filter_all_conv0}), 
		filters in this layer present characteristics more related to their own tasks.
	}
	\label{fig:filter_all_conv2}
	\vspace*{0mm}
\end{figure*}

\begin{figure*}[h]
	\begin{center}
		\vspace*{-3mm}
		%\fbox{\rule{0pt}{4.45in} \rule{1\linewidth}{0pt}}
		\includegraphics[width=0.85\linewidth]{figs/denoise_conv0.png}
		\caption{Filters with continuous changes for the \textit{feature extraction layer} (the first layer) in 
		denoising task. Numbers below show the correlation index for each filter with the first N20 filter.
		}
		\label{fig:denoise_conv0}
	\end{center}
\end{figure*}

\begin{figure*}[h]
	\begin{center}
		\vspace*{-3mm}
		%\fbox{\rule{0pt}{4.45in} \rule{1\linewidth}{0pt}}
		\includegraphics[width=0.85\linewidth]{figs/denoise_conv2.png}
		\caption{Filters with continuous changes for the \textit{reconstruction layer} (the last layer) in 
			denoising task. Numbers below show the correlation index for each filter with the first N20 filter.
		}
		\label{fig:denoise_conv2}
	\end{center}
\end{figure*}

\begin{figure*}[h]
	\begin{center}
		\vspace*{-3mm}
		%\fbox{\rule{0pt}{4.45in} \rule{1\linewidth}{0pt}}
		\includegraphics[width=0.85\linewidth]{figs/SR_conv2.png}
		\caption{Filters with continuous changes for the \textit{reconstruction layer} (the last layer) in 
			super-resolution task. Numbers below show the correlation index for each filter with the first K3 filter.
		}
		\label{fig:SR_conv2}
	\end{center}
\end{figure*}

\begin{figure*}[h]
	\begin{center}
		\vspace*{-3mm}
		%\fbox{\rule{0pt}{4.45in} \rule{1\linewidth}{0pt}}
		\includegraphics[width=0.85\linewidth]{figs/DeJPEG_conv2.png}
		\caption{Filters with continuous changes for the \textit{reconstruction layer} (the last layer) in 
			DeJPEG task. Numbers below show the correlation index for each filter with the first Q50 filter.
		}
		\label{fig:DeJPEG_conv2}
	\end{center}
\end{figure*}

\fi
